# Supplementary material for: Data augmentation for models based on rejection sampling
Source: arXiv:1406.6652 source file (2015-08-03)
Supplement: Supplementary file 1 [file appendix.tex]

Proof of Theorem \ref{th-weakConsistency}.

\begin{proof}

 The main ideas of proving consistency \citep[from][]{schwarz} are to bound the numerator of equation \eqref{eq-posteq} from above and the denominator from
below.  In order to bound the numerator, we construct uniformly consistent tests which separate the true density from its complement.
A condition on the prior mass of the Kullback-Leiber neighborhood of the true density is imposed to lower bound the denominator.  For weak consistency, it suffices to check  that the prior $\Pi$ assigns positive mass to any KL neighborhood of $f_0$ with which one can identify neighborhoods of $f_0$ for which uniformly consistent tests exist.

By slight abuse of notation, let denote $f$ as any continuous function on $\cM$ in this proof.  From \cite{abs2} the following conditions are sufficient to verify that the KL support condition holds.  \begin{itemize}
\item [(1)] The kernel $g(X,G,\boldsymbol{\kappa}) $ is continuous in all of its arguments.
\item [(2)] The set $\{F_0\}\times D_{\epsilon}^{o}$ intersects the support of $\Pi_1 \times \pi_{\bkappa}$ with $D_{\epsilon}^{o}$ as the interior of $D_{\epsilon}$,
which is a compact neighborhood of some $\{{\kappa}_1,\ldots, {\kappa}_p  \}$ in $\mathbb {R}^p$.
\item [(3)] For any continuous function $f$ on $M$, there exists a compact neighborhood $D_{\epsilon}$ of $\{{\kappa}_1,\ldots, {\kappa}_p  \}$, such that
\begin{align*}
\sup_{X\in V_{p,d},\;\boldsymbol\kappa\in D_{\epsilon} } \bigg\|f(X)-\int g(X, G, \boldsymbol \kappa)f(G)\lambda (dG)\bigg\|\leq \epsilon.
\end{align*}
\end{itemize}

We first verify condition (1).
Note that one can write
\begin{align*}
g(X, G, \boldsymbol \kappa)&=C(\boldsymbol{\kappa})\etr(F^TX)= C(\boldsymbol{\kappa})\exp\left(\sum_{i=1}^p\kappa_i G_{[:i]}^TX_{[:i]}  \right).
\end{align*}
$g$ is continuous with respect to $\boldsymbol \kappa$ since the hypergeometric function $C(\boldsymbol \kappa)$ is continuous and  $\etr(F^TX)$ is clearly continuous with respect to $\boldsymbol{\kappa}$ as the exponential term can be viewed as a linear combination of $\kappa_i$'s.

Now rewrite the density as
\begin{align*}
g(X, G, \boldsymbol \kappa)=C(\boldsymbol{\kappa})\etr(F^TX)=C(\boldsymbol{\kappa})\exp\left(\dfrac{p+\sum_{i=1}^p \kappa_i^2-\rho(F, X)^2}{2} \right),
\end{align*}
where $\rho$ is the Frobenius distance between two matrices $F$ and $X$. Therefore $\etr(F^TX)$ is a continuous density of $X$ with respect to the Frobenius distance. As mentioned in section 2, $V_{p,d}$ can be embedded  onto the Euclidean space $M(d,p)$ via the inclusion map. Therefore, one can equip $V_{p, d}$ with a metric space structure via the extrinsic distance $\rho$ in the Euclidean space.
From the symmetry between $G$ and $X$, $g$ is also continuous with respect to $G$.

To prove (2), note that DP  has weak support on all the measures  whose support is contained by the base measure $P_0$
(See Theorem 3.2.4 in \cite{jk}, pp. 104). As $P_0$ and $\pi_{\bkappa}$ have full support, (2) follows immediately.

Let $I(X)=f(X)-\int g(X, G, \boldsymbol \kappa)f(G)\lambda (dG)$.  For the last condition, we must show that there exists
some compact subset in $\mathbb R^p$ with non-empty interior, $D_{\epsilon}$, such that
\begin{equation}
\sup_{X\in V_{p,d},\;\boldsymbol\kappa\in D_{\epsilon} } \|I(X)\|\leq \epsilon.
\end{equation}

%Denote  $v (dX)$ as the volume form on the Stiefel manifold. The uniform distribution on $V_{p,d}$ has constant density $1/\int_{V_{p,d}}v(dX)$. The measure $\lambda$ on $V_{p,d}$ can be defined as $\lambda(S)=\int_S v(dX)$ for any measurable set $S$ on the Stiefel manifold.  Let $G_1$ be the matrix of size $d\times (d-p)$ such that $[G: G_1]$ is in $O(d)$, the group of orthogonal matrices.  One can represent $\lambda(dG)$ as $\wedge_{i=1}^p\wedge_{j=i+1}^{d}g_j^Tdg_i$ where $g_1,\ldots,g_p$ are the columns of $G$ and $g_{p+1},\ldots, g_d$ are the columns of $G_1$.

From symmetry of $g$ with respect to $G$ and $X$, one can rewrite
\begin{align*}
I(X)&=C(\boldsymbol \kappa)\int \left(f(X)-f(G)\right)\etr(F^TX)\lambda(dG).
\end{align*}
Let $\widehat{G}=Q(d)^TG$ where $Q(d)$ is an orthogonal matrix with first $p$ columns being $X$. Then $G=Q(d)\widehat{G}$. As the volume form is invariant under the group action of the orthogonal matrices $O(d)$ on the left, then one has $\lambda(dG)=\lambda(d\widehat{G})$.
First note that
\begin{align*}
\rho^2(X, Q(d)\widehat{G})&=\Tr\left( \left(X-  Q(d)\widehat{G}\right)\left(X- Q(d)\widehat{G}\right)^T \right)\\
&=2p-2\Tr\left(  Q(d)^TX\widehat{G}^T \right)\\
&=2 \sum_{i=1}^p \left(1-\widehat{g}_{ii} \right),
\end{align*}
with $\widehat{g}_{ii}$ being the diagonal elements of $\widehat{G}$.
%One makes a change of variables by l
Let $(1-\widehat{g}_{ii})=\frac{1}{\kappa_i}s_{ii}$ for $i=1,\ldots,p$, with $s_{ii}\in [0, 2\kappa_i]$.
Then $\rho^2(X, Q(d)\widehat{G})=2\sum_{i=1}^p \frac{1}{\kappa_i}s_{ii}.$
As $\kappa_i\rightarrow \infty$ for all $i=1,\ldots, p$,  $\rho^2(X, Q(d)\widehat{G})\rightarrow 0$.
Since $f$ is continuous and the Stiefel manifold is compact, one has for any $\boldsymbol{s}=\{s_{11},\ldots, s_{pp}\}$,
\begin{align}
\label{eq-c1}
\sup_{X\in V_{p,d}} \left|\left(f(X)-f(Q(d)\widehat{G})\right)\right|\rightarrow 0,
\end{align}
as $\kappa_i\rightarrow \infty$ for all $i=1,\ldots, p$.
Let $\widehat{F}$ be the matrix whose $k$th column is $\kappa_kQ(d)\widehat{G}_{[:k]}.$  One has
\begin{align}
\label{eq-supterm}
\sup_{X\in V_{p,d}} |I(X)|&\nonumber\leq \sup_{X\in V_{p,d}}C(\boldsymbol \kappa)\int \left|\left(f(X)-f(Q(d)\widehat{G})\right)\right|\etr(\widehat{F}^TX)\lambda(d\widehat{G})\\ \nonumber
&\leq C(\boldsymbol \kappa)\int \left\{\sup_{X\in V_{p,d}} \left|\left(f(X)-f(Q(d)\widehat{G})\right)\right|\right\}\exp\left(\sum_{i=1}^p\kappa_i\widehat{g}_{ii} \right)\lambda(d\widehat{G})\\
&=C(\boldsymbol \kappa)\exp\left(\sum_{i=1}^p\kappa_i\right)\int \left\{\sup_{X\in V_{p,d}} \left|\left(f(X)-f(Q(d)\widehat{G})\right)\right|\right\}\exp\left(-\sum_{i=1}^p s_{ii} \right)\lambda(d\widehat{G}).
%&=C(\boldsymbol \kappa)\exp\left(\sum_{i=1}^p\kappa_i\right)\int \left\{\sup_{X\in V_{p,d}} \left|\left(f(X)-f(Q(d)\widehat{G})\right)\right|\right\}\\
%&\exp\left(\sum_{i=1}^p-s_{ii} \right)\prod_{i=1}^p\dfrac{1}{\kappa_i}\lambda(d\widehat{G_s}),
\end{align}
Let $\pi_1$ be the transformation given by $\pi_1(\widehat{g}_{ij})=\widehat{g}_{ij}$ when $i\neq j$ and $\pi_1(\widehat{g}_{ii})=s_{ii}=\kappa_i(1-\widehat{g}_{ii}).$ Denote $\pi_2$ as the transformation of $\widehat{G}$ given by $\pi_2(\widehat{g}_{ii})=(1-\widehat{g}_{ii})$ and  $\pi_2(\widehat{g}_{ij})=\widehat{g}_{ij}$ when $i\neq j$ . Let $J_1$ and $J_2$ be the Jacobian corresponding to $\pi_1^{-1}$ and $\pi_2^{-1}$ respectively. Denote $\lambda(d\widehat{G_s})$ as new volume measure after changing of variables with respect to $\pi_1$. Rewrite $\lambda(d\widehat{G})=\varphi(\widehat{G})d\widehat{g}_{11}\wedge d\widehat{g}_{12}\cdots\wedge\widehat{g}_{dp}$ where $\varphi(\widehat{G})$ is some function of $\widehat{G}$.  Then $\lambda(d\widehat{G_s})$ is given by the pullback of $\lambda(d\widehat{G})$ induced by the map $\pi_1^{-1}$, that is
\begin{align}
\lambda(d\widehat{G}_s)=(\pi_1^{-1})^{*}(\lambda(d\widehat{G}))=\varphi(\pi_1^{-1}(\widehat{G}_s))\det(J_1)ds_{11}\wedge ds_{12}\cdots \wedge ds_{dp},
\end{align}
where $s_{ij}$ is the $(i,j)$th element of $\widehat{G}_s$.
Thus
\begin{align}
\lambda(d\widehat{G}_s)=\varphi(\pi_1^{-1}(\widehat{G}_s))\det(J_1)\det(J_2)\prod_{i=1}^p\kappa_id\widehat{g}_{11}\wedge d\widehat{g}_{12}\cdots \wedge d\widehat{g}_{dp},
\end{align}
which implies
\begin{align}
\label{eq-45}
\lambda(d\widehat{G})=1/\prod_{i=1}^p\kappa_i\frac{1}{\det(J_1)\det(J_2)}\lambda(dG_s).
\end{align}
Then the last term of \eqref{eq-supterm} becomes
\begin{align}
&\nonumber C(\boldsymbol \kappa)\exp\left(\sum_{i=1}^p\kappa_i\right)\prod_{i=1}^p\dfrac{1}{\kappa_i}\int \left\{\sup_{X\in V_{p,d}} \left|\left(f(X)-f(Q(d)\widehat{G})\right)\right|\right\}\times\\
&\exp\left(\sum_{i=1}^p-s_{ii} \right)\frac{1}{\det(J_1)\det(J_2)}\lambda(d\widehat{G_s}).
\end{align}
It is not hard  to see that
\begin{equation}\int \exp\left(-\sum_{i=1}^p s_{ii} \right)\frac{1}{\det(J_1)\det(J_2)}\lambda(d\widehat{G_s})<\infty.
\end{equation}

We now proceed to show that even as $\kappa_i \rightarrow \infty$,
\begin{equation}
C(\boldsymbol \kappa)\exp\left(\sum_{i=1}^p\kappa_i\right)\prod_{i=1}^p\dfrac{1}{\kappa_i}<\infty.
\end{equation}
One has
\begin{align*}
C(\boldsymbol \kappa)\exp\left(\sum_{i=1}^p\kappa_i\right)\prod_{i=1}^p\dfrac{1}{\kappa_i}
%&=1/_{0}F_1\left(\frac{1}{2}d, \frac{1}{4}\diag \left\{\kappa_1^2,\ldots, \kappa_p^2  \right\}\right)\prod_{i=1}^p\dfrac{\exp(\kappa_i)}{\kappa_i}\\
&=\dfrac{\prod_{i=1}^{p}\dfrac{1}{\kappa_i}}{_{0}F_1\left(\frac{1}{2}d, \frac{1}{4}\diag \left\{\kappa_1^2,\ldots, \kappa_p^2  \right\}\right)/\prod_{i=1}^p\exp(\kappa_i)}.
\end{align*}
Write (see \cite{bultler})
\begin{equation}
_{0}F_1\left(\frac{1}{2}d, \frac{1}{4}\diag \left\{\kappa_1^2,\ldots, \kappa_p^2  \right\}\right)=\int _{O_p}\etr\left(\diag \left\{\kappa_1,\ldots, \kappa_p  \right\}T  \right)dT
\end{equation}
with $T\in O_p$ the group of all the $p$ by $p$ orthogonal matrices with $dT$ given by $\wedge_{i<j}t_j^Tdt_i$.
When $\kappa_i\geq 1$ for $i=1,\ldots,p$, one looks at
\begin{align*}
\int _{O_p}\frac{\etr\left(\diag \left\{\kappa_1,\ldots, \kappa_p  \right\}T  \right)}{\prod_{i=1}^p\exp(\kappa_i)}dT&=\int_{O_p}\exp\left(-\left(\sum_{i=1}^p \kappa_i(1-t_{ii})  \right)\right)dT,
\end{align*}
where $t_{ii}$ are the diagonal elements of $T$. Let $u_{ii}=\kappa_i(1-t_{ii})$, one has $u_{ii}\in [0, 2\kappa_i]$. Let $d\widehat{T}$ be the volume form after changing of variable. By the same argument given in \eqref{eq-45},  we have
\begin{align*}
\int_{O_p}\exp\left(-\left(\sum_{i=1}^p \kappa_i(1-t_{ii})  \right)\right)dT=\prod_{i=1}^p1/\kappa_i\int \exp\left(-\left(\sum_{i=1}^p u_{ii}  \right)\right)\frac{1}{\det(J_3)\det(J_4)}d\widehat{T},
\end{align*}
where $\det(J_3)$ and $\det(J_4)$ corresponding to determinants of the Jacobian of maps $\pi_3$ and $\pi_4$ which are essentially the same maps as $\pi_1$ and $\pi_2$ but with domain $T\in O_p$.
Note $\int \exp\left(-\left(\sum_{i=1}^p u_{ii}  \right)\right)\frac{1}{\det(J_3)\det(J_4)}d\widehat{T}$ is bounded away from zero and infinity as $\kappa_i\rightarrow \infty$. Therefore, we can conclude
\begin{equation}
\label{eq-c2}
C(\boldsymbol \kappa)\exp\left(\sum_{i=1}^p\kappa_i\right)\prod_{i=1}^p\dfrac{1}{\kappa_i}<\infty.
\end{equation}
Therefore, combining \eqref{eq-c1} and \eqref{eq-c2} and by the dominated convergence theorem, one has
\begin{align*}
\sup_{X\in V_{p,d}} |I(X)|\rightarrow 0
\end{align*}
as $\kappa_i\rightarrow \infty$ for all $i=1,\ldots, p$. Thus  for all $\epsilon>0$, there exists $M_i$ large enough such that, when $\kappa_i>M_i$, $\sup_{X\in V_{p,d}} |I(X)|\leq \epsilon$. One can take $D_{\epsilon}$ to be a $\epsilon$ neighborhood of $\{\kappa_1,\ldots, \kappa_p\}$ with $\kappa_i>\max\{M_i,i=1,\ldots, p\}$.
\end{proof}

%%%%%%%%%%%%%%%%%%%%%%%%%%%%%%%%%%%%%%%%%%%%%%%%%%%%%%%%%%%%%%%%%%%%%%%%%%%%%%%%%%%%%%%%%%%%%%%%%%%%%%%%%%%%%%%%%%%%%%%%%%%%%%%%%%%%%%%%%%%%%%%%%%%

Proof of Theorem \ref{th2}.

\begin{proof}
In order to establish strong consistency, it is not sufficient for the prior $\Pi$ to assign positive mass to any Kullback-Leibler neighborhood of $f_0$. %In order to verify tests condition,
We need to construct high mass sieves with   metric entropy $N(\epsilon, \mathcal{F})$ bounded by certain order where $N(\epsilon, \mathcal{F})$  is defined as the logarithm of the
minimum number of balls with Hellinger radius $\epsilon$ to cover the space $\mathcal{F}$.  We refer to \cite{barron} for some general strong consistency theorems.
We first proceed to verify the following two conditions on the kernel $g(X,G, \boldsymbol{\kappa})$.
\begin{itemize}
\item [(a)] There exists positive constants $k_0$, $a_1$ and $A_1$ such that for all $k>k_0$, $G_1,G_2\in V_{p,d}$ one has
\begin{equation}
\label{eq-ca}
\sup_{X\in V_{p,d}, \boldsymbol{\kappa}\in \phi^{-1}[0,k]} |g(X,G_1,\boldsymbol{\kappa})-g(X,G_2,\boldsymbol{\kappa})|\leq A_1k^{a_1}\rho (G_1,G_2),
\end{equation}
where $\phi: \mathbb R^{p}\rightarrow [0,\infty)$ is some  continuous function of $\boldsymbol{\kappa}$.
\item [(b)] There exists positive constants $a_2$ and $A_2$ such that for all $\boldsymbol{\kappa}, \widetilde{\boldsymbol{\kappa}} \in \phi^{-1}[0,k]$, $k\geq k_0$,
\begin{equation}
\label{eq-cb}
\sup_{X, G\in V_{p,d}} |g(X,G,\boldsymbol{\kappa})-g(X,G,\widetilde{\boldsymbol{\kappa}})|\leq A_2k^{a_2}\rho_2 (\boldsymbol{\kappa},\widetilde{\boldsymbol{\kappa}}),
\end{equation}
where $\rho_2$ is the Euclidean distance $\|\cdot\|_2$ on $\mathbb{R}^p$.
\end{itemize}

Let $G_1, G_2\in V_{p,d}$ and $F_1$ and $F_2$ be such that their $i$th columns are given by $\kappa_iG_{1_{[:,i]}}$ and $\kappa_iG_{2_{[:,i]}}$ respectively.
For $s, t\in [0,c] $  and $c>0$, one has
\begin{align*}
\Big|\exp\left(-\frac{s^2}{2}\right)-\exp\left(-\frac{t^2}{2}\right)\Big|\leq \Big|\eta\exp\left(-\frac{\eta^2}{2}\right)(s-t)\Big|\leq c |s-t|,
\end{align*}
where $\eta$ is some point between $s$ and $t$.
 Let $k_{\max}=\max\{\kappa_1,\ldots, \kappa_p\}$. A little calculation shows that $\rho(F,X)\leq \sqrt{\sum_{i=1}^p (\kappa_i+1)^2}$, so that
\begin{align*}
&\sup_{X\in V_{p,d}, \boldsymbol{\kappa}\in \phi^{-1}[0,k]} \bigg|g(X,G_1,\boldsymbol{\kappa})-g(X,G_2,\boldsymbol{\kappa})\bigg|\\
&=\sup_{X\in V_{p,d}, \boldsymbol{\kappa}\in \phi^{-1}[0,k]}\bigg|C(\boldsymbol{\kappa})\exp \left(\frac{p}{2}\right)\exp\left(\frac{\sum_{i=1}^{p}\kappa_i}{2}  \right)\left(\exp\left(-\frac{\rho^2(F_1,X)}{2}\right)- \exp\left(-\frac{\rho^2(F_2,X)}{2}\right) \right)\bigg|\\
&\leq \sup_{X\in V_{p,d}, \boldsymbol{\kappa}\in \phi^{-1}[0,k]}\bigg|C(\boldsymbol{\kappa})\exp \left(\frac{p}{2}\right)\exp\left(\frac{\sum_{i=1}^{p}\kappa_i}{2}  \right)\sqrt{\sum_{i=1}^p (\kappa_i+1)^2}\left(\rho(F_1,X)-\rho(F_2,X)\right)\bigg|\\
&\leq \exp \left(\frac{p}{2}\right)\sup_{X\in V_{p,d}, \boldsymbol{\kappa}\in \phi^{-1}[0,k]}\bigg|C(\boldsymbol{\kappa})\exp\left(\frac{\sum_{i=1}^{p}\kappa_i}{2}  \right)\rho(F_1,F_2)\sqrt{\sum_{i=1}^p (\kappa_i+1)^2}\bigg|\\
&\leq 2\exp \left(\frac{p}{2}\right)\sup_{X\in V_{p,d}, \boldsymbol{\kappa}\in \phi^{-1}[0,k]}\bigg|C(\boldsymbol{\kappa})\exp\left(\frac{\sum_{i=1}^{p}\kappa_i}{2}  \right)\sqrt{\sum_{i=1}^p\kappa_i^2}\rho(G_1,G_2)\sqrt{\sum_{i=1}^p (\kappa_i+1)^2}\bigg|\\
&\leq 2\exp \left(\frac{p}{2}\right)\sup_{X\in V_{p,d}, \boldsymbol{\kappa}\in \phi^{-1}[0,k]}\bigg| C\prod_{i=1}^p\kappa_i\sqrt{\sum_{i=1}^p\kappa_i^2}\sqrt{\sum_{i=1}^p (\kappa_i+1)^2} \rho(G_1,G_2)\bigg|
\end{align*}
where $C$ is some constant according to \eqref{eq-c2}.
Let $\phi(\boldsymbol{\kappa})=\sqrt{\sum_{i=1}^p (\kappa_i+1)^2}$. If $\phi(\boldsymbol{\kappa})\leq k$, then
$\sqrt{\sum_{i=1}^p\kappa_i^2}\leq \phi(\boldsymbol{\kappa})\leq k$ and $\kappa_i\leq k$ for each $i$. Thus $\prod_{i=1}^p\kappa_i\leq k^p$. Therefore,
\begin{align*}
\sup_{X\in V_{p,d}, \boldsymbol{\kappa}\in \phi^{-1}[0,k]} |g(X,G_1,\boldsymbol{\kappa})-g(X,G_2,\boldsymbol{\kappa})|\leq C_1k^{p+2}\rho(G_1,G_2),
\end{align*}
with $C_1$ some constant.
Let $a_1=p+2$, then condition (a) holds.

Let $\boldsymbol{\kappa}$, $\widetilde{\boldsymbol{\kappa}}\in \mathbb R^p$ be two vectors of the concentration parameters.
By the mean value theorem, one has for some $t\in (0,1)$
\begin{align*}
g(X,G,\boldsymbol{\kappa})-g(X,G,\widetilde{\boldsymbol{\kappa}})=\left(\bigtriangledown g(X,G, (1-t)\boldsymbol{\kappa}+t\widetilde{\boldsymbol{\kappa}})\right)\cdot(\boldsymbol{\kappa}-\widetilde{\boldsymbol{\kappa}}),
\end{align*}
where $\bigtriangledown g(X,G, (1-t)\boldsymbol\kappa+t\widetilde{\boldsymbol{\kappa}})$ is the gradient of $g(X,G, \boldsymbol\kappa)$ with respect to $\boldsymbol{\kappa}$ evaluated at $(1-t)\boldsymbol\kappa+t\widetilde{\boldsymbol{\kappa}}$  and $\cdot$ denotes the inner product.
By Cauchy-Schwarz inequality, one has
\begin{align*}
 |g(X,G,\boldsymbol{\kappa})-g(X,G,\widetilde{\boldsymbol{\kappa}})|\leq \| \bigtriangledown g(X,G, (1-t)\boldsymbol\kappa+t\widetilde{\boldsymbol{\kappa}}) \|_2  \| \boldsymbol{\kappa}-\widetilde{\boldsymbol{\kappa}}  \|_2.
\end{align*}
Note that  for $i=1,\ldots, p$,
\begin{align*}
\dfrac{\partial g}{\partial \kappa_i}&=\exp\left(-\sum_{i=1}^p \kappa_i(1-G_{[:i]}^TX_{[:i]} )\right) \left(C(\boldsymbol{\kappa})G_{[:i]}^TX_{[:i]}\exp(\sum_{i=1}^p\kappa_i)+\dfrac{\partial C(\boldsymbol{\kappa})}{\partial \kappa_i} \exp(\sum_{i=1}^p\kappa_i) \right)\\
%&=\exp\left(-\sum_{i=1}^p \kappa_i(1-H_{[:i]}^TX_{[:i]} )\right) \left(C(\boldsymbol{\kappa})H_{[:i]}^TX_{[:i]}\exp(\sum_{i=1}^p\kappa_i)+\dfrac{\partial C(\boldsymbol{\kappa})}{\partial \kappa_i}\exp(\sum_{i=1}^p\kappa_i)  \right)\\
&=\exp\left(-\sum_{i=1}^p \kappa_i(1-G_{[:i]}^TX_{[:i]} )\right) \bigg(C(\boldsymbol{\kappa})G_{[:i]}^TX_{[:i]}\exp(\sum_{i=1}^p\kappa_i)\\
&-C^2(\boldsymbol{\kappa})\dfrac{\partial _{0}F_1\left(\frac{1}{2}d, \frac{1}{4}\diag \left\{\kappa_1^2,\ldots, \kappa_p^2  \right\}\right)}{\partial \kappa_i}\exp(\sum_{i=1}^p\kappa_i)\bigg).
\end{align*}

By applying the general Leibniz rule for differentiation under an integral sign, one has
\begin{align*}
\dfrac{\partial _{0}F_1\left(\frac{1}{2}d, \frac{1}{4}\diag \left\{\kappa_1^2,\ldots, \kappa_p^2  \right\}\right)}{\partial \kappa_i}&=\int _{O_p}\dfrac{\partial\etr\left(\diag \left\{\kappa_1,\ldots, \kappa_p  \right\}S  \right)}{\partial \kappa_i}dS\\
&=\int _{O_p}s_{ii} \exp \left(\sum_{i=1}^p\kappa_is_{ii}\right)dS\\
&\leq \int _{O_p} \exp \left(\sum_{i=1}^p\kappa_is_{ii}\right)dS=\dfrac{1}{C(\boldsymbol{\kappa})}.
\end{align*}
Then one has \begin{align*}
\left|\dfrac{\partial g(X,G,\boldsymbol{\kappa})}{\partial \kappa_i}\right|&\leq C(\boldsymbol{\kappa})\exp\left(\sum_{i=1}^p\kappa_i\right)+C^2(\boldsymbol{\kappa})\dfrac{\partial _{0}F_1\left(\frac{1}{2}d, \frac{1}{4}\diag \left\{\kappa_1^2,\ldots, \kappa_p^2  \right\}\right)}{\partial\kappa_i}\exp\left(\sum_{i=1}^p\kappa_i\right)\\
&\leq 2C(\boldsymbol{\kappa})\exp\left(\sum_{i=1}^p\kappa_i\right)\leq C_2\prod_{i=1}^p\kappa_i,
\end{align*}
for some constant $C_2$ by \eqref{eq-c2}.
Therefore,
\begin{align*}
 \| \bigtriangledown g(X,G, (1-t)\boldsymbol\kappa+t\widetilde{\boldsymbol{\kappa}}) \|_2\leq C_2k^{p}.
\end{align*}
Then one has
\begin{align*}
 |g(X,G,\boldsymbol{\kappa})-g(X,G,\widetilde{\boldsymbol{\kappa}})|\leq C_2k^p \| \boldsymbol{\kappa}-\widetilde{\boldsymbol{\kappa}}  \|_2.
\end{align*}
Letting $a_2=p$, condition (b) is verified.

We proceed to verify the two following entropy conditions:
\begin{itemize}
\item [(c)] For any $k\geq k_0$, the subset $\phi^{-1}[0, k]$ is compact and its $\epsilon$-covering number is bounded by $(k\epsilon^{-1})^{b_2}$ for some constant $b_2$ independent of $\boldsymbol{\kappa}$ and $\epsilon$.

\item [(d)] The $\epsilon$ covering number of the manifold $V_{p,d}$ is bounded by $A_3\epsilon^{-a_3}$ for any $\epsilon>0$.
\end{itemize}
It is easy to verify condition (c) as $\phi^{-1}([0,k])=\{\boldsymbol{\kappa}, \sum_{i=1}^p(\kappa_i+1)^2\leq k^2  \}$, which is a subset of a shifted Euclidean ball in $\mathbb R^p$ with radius $k$. With a direct argument using packing numbers \citep[see Section 4]{pollard},
one can obtain a  bound for the entropy of $\phi^{-1}[0,k]$ which is given by $\dfrac{3k^p}{\epsilon^p}$. Thus condition (c) holds with $b_2=p$.

%Now one looks at the entropy number of $V_{p,d}$.
Denote $N(\epsilon)$ as the entropy of $V_{p,d}$ and $N_{E}(\epsilon)$ as the entropy of $V_{p,d}$ viewed as a subset of $\mathbb R^{pd}$
(thus points covering $V_{p,d}$ do not necessarily lie on $V_{p,d}$ for the latter case). One can show that $N(2\epsilon)\leq N_{E}(\epsilon)$.
Note that $V_{p,d}\subset[-1,1]^{pd}$ which is a subset of a Euclidean ball of radius $\sqrt{dp}$ centered at zero, the $\epsilon$ number of which is bounded $\left(\dfrac{3\sqrt{dp}}{\epsilon}\right)^{dp}$. Therefore, condition (d) holds with $a_3=dp$.  Then by Corollary 1 in \cite{abs2}, strong consistency follows.

\end{proof}
